# Supplementary material for: Human-in-the-Loop Methods for Data-Driven and Reinforcement Learning Systems
Source: arXiv:2008.13221 source file (2020-08-30)
Supplement: Supplementary file 2 [file appendix1.tex]

%%%%%%%%%%%%%%%%%%%%%%%%%%%%%%%%%%%%%%%%%%%%%%%%%%%
%
%  New template code for TAMU Theses and Dissertations starting Fall 2016.
%
%
%  Author: Sean Zachary Roberson 
%	 Version 3.16.09
%  Last updated 9/12/2016
%
%%%%%%%%%%%%%%%%%%%%%%%%%%%%%%%%%%%%%%%%%%%%%%%%%%%

%%%%%%%%%%%%%%%%%%%%%%%%%%%%%%%%%%%%%%%%%%%%%%%%%%%%%%%%%%%%%%%%%%%%%%
%%                           APPENDIX A 
%%%%%%%%%%%%%%%%%%%%%%%%%%%%%%%%%%%%%%%%%%%%%%%%%%%%%%%%%%%%%%%%%%%%%

\phantomsection

\chapter{\uppercase{First Appendix}}

Text for the Appendix follows.

\begin{figure}[h]
\centering
\includegraphics[scale=.50]{figures/Penguins.jpg}
\caption{TAMU figure}
\label{fig:tamu-fig5}
\end{figure}
